# Supplementary material for: NVDiff: Graph Generation through the Diffusion of Node Vectors
Source: arXiv:2211.10794 source file (2023-06-20)
Supplement: Supplementary file 4 [file chemical-appendix-qm9.tex]

\begin{table}[h]
    \centering
    \small
    \caption{NVDiffs' performance on QM9 when trained with 10\% of the data. Novelty and Novelty(100\%) denote the novelty metrics calculated over the training set and the whole dataset, respectively.}
    \label{tab:qm9-ten}
    \begin{tabular}{l|cccccc}\hline
         & Validity$\uparrow$ & Uniqueness$\uparrow$ & Novelty$\uparrow$ & Novelty(100\%)$\uparrow$ &NSPDK$\downarrow$ & FCD$\downarrow$ \\\hline
        NVDiff &90.29$\pm$1.12&94.88$\pm$0.96&99.99$\pm$0.002&57.51$\pm$2.12&0.003$\pm$0&1.758$\pm$0.39\\
         NVDiff-E &97.36$\pm$0.96&97.63$\pm$0.65&98.61$\pm$0.016&59.74$\pm$1.84&0.001$\pm$0&0.989$\pm$0.11\\ \hline
    \end{tabular}
\end{table}
